# Supplementary material for: A stacked approach for chained equations multiple imputation incorporating the substantive model
Source: arXiv:1910.04625 ancillary file (2019-10-10)
Supplement: Supplementary file 1 [file Supplementary_Materials.pdf]

# Web Appendix to "A stacked approach for chained equations multiple imputation incorporating the substantive model"

**Lauren J. Beesley*[1] and Jeremy M G Taylor[1]**
[1]University of Michigan, Department of Biostatistics
*Corresponding Author: lbeesley@umich.edu

## 1 Derivation of proposed variance estimator

In this section, we motivate our estimator for standard errors after analyzing data from stacked multiple imputation (with weights). This estimator can be applied when we routinely impute data using MICE and then stack with weights defined as 1 over the number of times each patient appears in the stacked dataset or when we define imputations and weights as in **Figure 1**.

We first observe that we are interested in estimating the observed data information matrix, $I_{obs}$. Following Louis (1982), we can express this as follows:

$$I_{obs}(\theta) = I_{com}(\theta) - I_{mis}(\theta)$$

where $I_{com}$ is the expected complete data information given the observed data and $I_{mis}$ is the expected missing information due to the missing data given the observed data. Let $J_{com}$ be the negative of the second derivative matrix of the complete data log-likelihood function. Let $U_{com}$ be the first derivative matrix of the complete data log-likelihood function. Following Louis (1982), we can rewrite this expression as follows:

$$\begin{aligned} I_{obs}(\theta) &= E_\theta(J_{com}(\theta)|X^{obs}, Y) - \left[E_\theta(U_{com}(\theta)^{\otimes 2}|X^{obs}, Y) - E_\theta(U_{com}(\theta)|X^{obs}, Y)^{\otimes 2}\right] \\ &= E_\theta(J_{com}(\theta)|X^{obs}, Y) - Var_\theta(U_{com}(\theta)|X^{obs}, Y) \end{aligned}$$

where the expectations are with respect to the distribution of the missing data. Now, we assume that data are independent across $i$. In this case, we can rewrite the above as

$$I_{obs}(\theta) = \sum_i E_\theta(J^i_{com}(\theta)|X^{obs}, Y) - \sum_i Var_\theta(U^i_{com}(\theta)|X^{obs}, Y)$$

where $J^i_{com}(\theta)$ and $U^i_{com}(\theta)$ are the contributions to the complete data information matrix and score matrix for patient $i$ respectively.

In practice, these conditional expectations and variances are not simple to calculate. However, we can approximate these expression as averages of these expressions evaluated across imputed datasets, which were imputed by drawing from distributions for the missing data given the observed data. A similar approach is used in the context of Monte Carlo log-likelihood maximization in Wei and Tanner (1990).

Suppose first that we give equal weight to multiple imputations within a particular patient. Let $X_{im}$ be the $m^{th}$ imputation of the missing covariates for patient $i$. For patients without missing values, define $X_{im}$ to be all equal to fully-observed $X_i$, and suppose we apply data analysis using the "tall stack" where each fully-observed patient appears in the stacked dataset $M$ times. A similar expression is also applicable for the "short stack" formulation, where each fully-observed patient appears only once in the stacked data. We can approximate the above

expression as follows:

$$I_{obs}(\theta) \approx \sum_i \frac{1}{M} \sum_m J^i_{com}(X_{im}, Y_i; \theta) - \sum_i \frac{1}{M} \sum_m \left[ U^i_{com}(X_{im}, Y_i; \theta) - \frac{1}{M} \sum_j U^i_{com}(X_{ij}, Y_i; \theta) \right]^{\otimes 2}$$

where $M$ is the number of multiple imputations. Now, suppose we give multiple imputations within patient $i$ unequal weight, where imputation $m$ for patient $i$ is given weight $w_{im}$, where $\sum_m w_{im} = 1$. We propose the following reformulation of the above approximation with unequal weights across multiple imputations within patients:

$$I_{obs}(\theta) \approx \sum_i \sum_m w_{im} J^i_{com}(X_{im}, Y_i; \theta) - \sum_i \sum_m w_{im} \left[ U^i_{com}(X_{im}, Y_i; \theta) - \bar{U}^i_{com}(X_i, Y_i; \theta) \right]^{\otimes 2}$$

where $\bar{U}^i_{com}(X, Y_i; \theta) = \sum_j w_{im} U^i_{com}(X_{ij}, Y_i; \theta)$. We can evaluate this expression at the maximum likelihood estimator for $\theta$, $\hat{\theta}$, obtained previously from fitting the model for $Y|X$ to the weighted, stacked dataset to obtain an estimate of the observed data information matrix. Inverting this matrix will provide the estimate for the observed data covariance matrix for $\hat{\theta}$ in *Eq. 2*.

## 2 Imputation strategy for linear regression

In order to make this estimation strategy clearer, we demonstrate how it works for linear regression. Suppose we are interested in fitting a linear regression model for outcome $Y$ using covariates $X$ and variance parameter $\sigma^2$. Suppose further that we have missing data in $X$, and we multiply impute these missing values using only other information in $X$ to obtain $X_{im}$ for each patient $i$ and imputations $m = 1, \ldots, M$.

Suppose we stack the $M$ imputed datasets on top of each other to create a dataset of size $Mn \times p$, where $p$ is the dimension of $X_i$. Using $\hat{\theta}_{cc}$ from fitting a linear regression model for $Y|X$ on the complete case data (patients with $X$ fully observed), we define weights

$$w_{im} = \frac{\frac{1}{\sqrt{2\pi\sigma^2_{cc}}} e^{-\frac{(Y_i - X_{im}\beta_{cc})^2}{2\sigma^2_{cc}}}}{\sum_{j=1}^{M} \frac{1}{\sqrt{2\pi\sigma^2_{cc}}} e^{-\frac{(Y_i - X_{ij}\beta_{cc})^2}{2\sigma^2_{cc}}}} = \frac{e^{-\frac{(Y_i - X_{im}\beta_{cc})^2}{2\sigma^2_{cc}}}}{\sum_{j=1}^{M} e^{-\frac{(Y_i - X_{ij}\beta_{cc})^2}{2\sigma^2_{cc}}}}$$

For subjects with fully-observed $X_i$, this express will equal $1/M$ for all $m$. Now, we define the complete data log-likelihood, score and information matrices (just focusing on the part based on $\beta$ as follows:

$$\begin{aligned}
l^i_{com}(X_{im}, Y_i; \theta) &= -\frac{(Y_i - X_{im}\beta)^2}{2\sigma^2} - \log\left[\sqrt{2\pi\sigma^2}\right] \\
U^i_{com}(X_{im}, Y_i; \theta) &= \frac{Y_i - X_{im}\beta}{\sigma^2} X_{im} \\
J^i_{com}(X_{im}, Y_i; \theta) &= \frac{X_{im}X_{im}^T}{\sigma^2}
\end{aligned}$$

so we have that

$$I_{obs}(\theta) \approx \sum_i \sum_m w_{im} \frac{X_{im}X_{im}^T}{\sigma^2} - \sum_i \sum_m w_{im} \left[\frac{Y_i - X_{im}\beta}{\sigma^2} X_{im} - \bar{U}^i_{com}(X_i, Y_i; \theta)\right]^{\otimes 2}$$

where $\bar{U}^i_{com}(X_i, Y_i; \theta) = \sum_j w_{ij} \frac{Y_i - X_{ij}\beta}{\sigma^2} X_{ij}$ and we then plug in the final maximum likelihood estimates for $\beta$ and $\sigma^2$ into the above expression.

# 3 Example R code for implementation

In this section, we provide some example R code to demonstrate how we can implement our proposed imputation approach. First, we provide some code to simulate outcome $Y$ and covariates $X$ and $B$ from a multivariate normal distribution. We then generate missingness in $B$ under missing completely at random (MCAR) assumptions with a 50% missingness rate.

We use *mice* in R to impute missing values of $B$, but we impute $B$ from a distribution that does *not* condition on $Y$. We then take these 50 imputed datasets and stack them. Weights are obtained by first fitting the outcome model (linear regression for $Y|X,B$) to the complete case dataset. We use the resulting parameter estimates to obtain weights proportional to $Y|X,B$. Weights are then scaled to sum to 1 across imputed datasets but within individuals. In the final estimation step, we fit a weighted version of the same regression model to the stacked data. We estimate corresponding standard errors using *Eq. 2* available in the R package *StackImpute*.

```
### Download R package from GitHub
devtools::install_github("lbeesleyBIOSTAT/StackImpute", build_vignettes = TRUE, build_
    opts = c("--no-resave-data", "--no-manual"))
library(StackImpute)

### Simulate Data
Nobs = 2000
DAT = MASS::mvrnorm(n = Nobs, mu = c(0,0,0), Sigma = rbind(c(1, 0.18, 0.42), c(0.18,
    0.09, 0.12),c(0.42, 0.12, 0.49 )))
Y = DAT[,1]
B = DAT[,2]
X = DAT[,3]
S = sample(x=c(0,1), size = Nobs, prob = c(0.5,0.5), replace = TRUE)
complete_cases = data.frame(Y, X, B, S)[S == 1,] #complete case subjects only
observed_data = data.frame(Y, X, B, S) #data with missingness in B
observed_data[S==0,'B'] = NA

### Step 1: Impute B|X
imputes = mice::mice(observed_data, m=50, method="norm", maxit = 1)
pred = imputes$predictorMatrix
pred[pred != 0] = 0
pred["B","X"] = 1
imputes = mice::mice(observed_data, m=50, predictorMatrix=pred, method="norm")

### Step 2: Stack imputed datasets
stack = mice::complete(imputes, action="long", include = FALSE)

### Step 3: Obtain weights
library(dplyr)
fit_cc = glm(Y ~ X + B, family='gaussian', data= complete_cases)
stack$wt = dnorm(stack$Y,mean = predict(fit_cc, newdata = stack), sd = sqrt(summary(fit_
    cc)$dispersion))
stack = as.data.frame(stack %>% group_by(.id) %>% mutate(wt = wt / sum(wt)))

### Step 4: Estimation
fit = glm(Y ~X + B, data=stack, family=gaussian(), weights = stack$wt)
Info = StackImpute::Louis_Information(fit, stack, M = 50, IMPUTED = unique(stack$.id[
    stack$S==0]))
VARIANCE = diag(solve(Info))
```

Alternatively, one can perform analysis using a short stack, where patients with complete case data only appear once and patients with missing data appear $M$ times as follows:

```
### Step 2: Stack imputed datasets
cc = unique(stack$.id[stack$S == 1])
stack_short = rbind(stack[stack$S==0,], stack[stack$S==1 & !duplicated(stack$.id),])

### Step 3: Obtain weights
stack_short$wt = dnorm(stack_short$Y,mean = predict(fit_cc, newdata = stack_short), sd =
     sqrt(summary(fit_cc)$dispersion))
stack_short = as.data.frame(stack_short %>% group_by(.id) %>% mutate(wt = wt / sum(wt)))

### Step 4: Estimation
fit = glm(Y ~X + B, data=stack_short, family=gaussian(), weights = stack_short$wt)
Info = StackImpute::Louis_Information(fit, stack_short, M = 50, IMPUTED = unique(stack_
    short$.id[stack_short$S==0]))
VARIANCE = diag(solve(Info))
```

## References


Thomas A Louis. Finding the Observed Information Matrix when Using the EM Algorithm. *Journal of the Royal Statistical Society*, 44(2):226–233, 1982.

Greg C G Wei and Martin A Tanner. A Monte Carlo Implementation of the EM Algorithm and the Poor Man's Data Augmentation Algorithms. *Journal of the American Statistical Association*, 85(411):699–704, 1990.
